# Supplementary material for: M3T: A New Benchmark Dataset for Multi-Modal Document-Level Machine Translation
Source: arXiv:2406.08255 source file (2024-06-12)
Supplement: Supplementary file 1 [file 8-appendix.tex]

\section{Training Hyperparameters}
